# Supplementary material for: Doubly-stochastic mining for heterogeneous retrieval
Source: arXiv:2004.10915 source file (2020-04-23)
Supplement: Supplementary file 1 [file appendix_cvar_concentration.tex]

\citet{Brown:2007} showed that as $n$ becomes large, for a continuous random variable $X$ with a bounded support, $\widehat{C}_{\alpha}$ concentrates arbitrarily close to $\cvar_{\alpha}(X)$ with high probability:

\begin{proposition}[\cite{Brown:2007}]
\label{prop:brown}
Let $X$ be a continuous random variable with ${\rm supp}(X) \subseteq [a, b]$.
Then, for every $\delta \in (0, 1)$,
\begin{align}
\label{eq:brown-upp}
&\Pr\bigg[\cvar_{\alpha}(X) \leq \widehat{C}_{\alpha}(X) + \frac{(b-a)}{\sqrt{\alpha}} \cdot \sqrt{\frac{5\ln(3/\delta)}{n}}\bigg] \geq 1 - \delta,\\
&\Pr\bigg[\cvar_{\alpha}(X) \geq \widehat{C}_{\alpha}(X) - \frac{(b-a)}{\alpha} \cdot \sqrt{\frac{\ln(1/\delta)}{2n}}\bigg] \geq 1 - \delta.
\label{eq:brown-lower}
\end{align}
\end{proposition}
Observe here the differing dependences on $\alpha$: while the upper bound has a dependence on $\alpha^{-1/2}$, the lower bound has a $\alpha^{-1}$ dependence.
In fact, \citet{WangGao:2010} established the following {\color{red}improved result}.%
\ankit{Not sure if this is an improved result. Check this!}
\aditya{I think it is better in terms of dependence on $\alpha$.}

\begin{proposition}[\cite{WangGao:2010}]
Let $X$ be a continuous random variable with ${\rm supp}(X) \subseteq [a, b]$. Then, we have
\begin{align}
& \Pr\bigg[\bigg | \widehat{C}_{\alpha}(X) - \cvar_{\alpha}(X)\bigg | \geq \epsilon \bigg] \leq 6 \exp\bigg(-\frac{\alpha \epsilon^2}{11(b-a)^2}n\bigg)
\end{align}
\end{proposition}

It follows from \eqref{eq:atopk-cvar} and Proposition~\ref{prop:brown} that as number of observations become large, the average {\rm top}-k loss aims to select $f\in \FCal$ such that the conditional value at risk at level $\alpha = \frac{k}{n}$ of $\ell(Y, f(X))$ is minimized.

A uniform deviation bound based on the above was provided in~\citet[Proposition IV.9]{Cherukuri:2019}, who showed that
\begin{align}
\label{eq:cvar-uniform-bound}
\Pr\bigg[ \sup_{f \in \FCal} | \cvar_{\alpha}( f( X ) ) - \widehat{C}_{\alpha}( f( X ) ) | > \epsilon \bigg] \leq \gamma( \epsilon ) \cdot e^{-n \cdot \beta( \epsilon )},
\end{align} 
where $\gamma( \epsilon ) = \mathscr{O}( \mathrm{diam}( \FCal ) \cdot (\epsilon \cdot \alpha)^{-1} )$, 
and $\beta( \epsilon ) = \mathscr{O}( \alpha \cdot \epsilon^2 \cdot \mathrm{diam}( C )^{-2} )$,
where $\mathrm{diam}( \FCal )$ is the diameter of the function class,
and $\mathrm{diam}( C )$ is the diameter of the CVaR values.
